# Supplementary material for: GarmentImage: Raster Encoding of Garment Sewing Patterns with Diverse Topologies
Source: arXiv:2505.02592 source file (2025-05-06)
Supplement: Supplementary file 1 [file appendix.tex]

\section{Deformation of a quad mesh in encoding}

This process deforms the quad mesh on the grid so that its boundary conforms to the piece boundary while minimizing the distortion of quad elements. We solve the following minimization problem to compute the vertex coordinates {v} of the mesh.

$$ 
v = argmin_v\{ \sum_{i,j \in E}((v_j-v_i) - (g_j-g_i)^2) + \sum_{i \in B} (v_i-b_i)^2 \} 
$$

where $E$ is the mesh edges, $B$ is the vertices on the boundary, $g_i$ is the position of $v_i$ on the grid before deformation, and $b_i$ is the position on the boundary curve associated with $v_i$. 
The first term minimizes the difference between edge vector before deformation and after deformation to keep the grid shapes. The second term minimizes the distance between mesh vertices and corresponding vertices on the boundary curves. 
This can be written in a matrix form $|Lx-B|^2$ for each dimension, and we obtain x as a solution of $(L^TL)x = L^TB$. We use umfpack [] to solve this sparse linear system.

\section{Deformation of a quad mesh in decoding}

This process deforms the quad mesh on the grid so that its edge vectors becomes as-close-as-possible to the embedded edge vectors.
We solve the following minimization problem to compute the vertex coordinates {v} of the mesh.

\begin{align}
v = \argmin_v (\sum_{i,j \in E}((v_j-v_i) - vec_{ij})^2) +  \sum_{i \in V}(v_i - g_i )^2 )
\end{align}
where $E$ is the mesh edges, $V$ is mesh vertices, $vec_{ij}$ is encoded edge vector, $g_i$ is the position of $v_i$ on the grid before deformation. The first term minimizes the difference between resulting edge vector and embedded edge vectors. The second term keeps the location of the resulting mesh on the grid. Again, This can be written in a matrix form $|Lx-B|^2$ for each dimension, and we obtain $x$ as a solution of $(L^TL)x = L^TB$.

\section{Sketch-to-Garment Model}

We used a standard U-net structure as shown in Figure. We used cross entropy loss for inside/outside labels and edge type labels. We used mean squared error for edge deformation vectors. We excluded edge type and  deformation outside regions from the loss computation, which significantly improved performance. We used Adam as optimizer. We trained the model for 1,000 epocs with all training data in a single batch. We applied random translation and scaling to input data as data augmentation.

\begin{figure}[h]
  \centering
  \includegraphics[width=\linewidth]{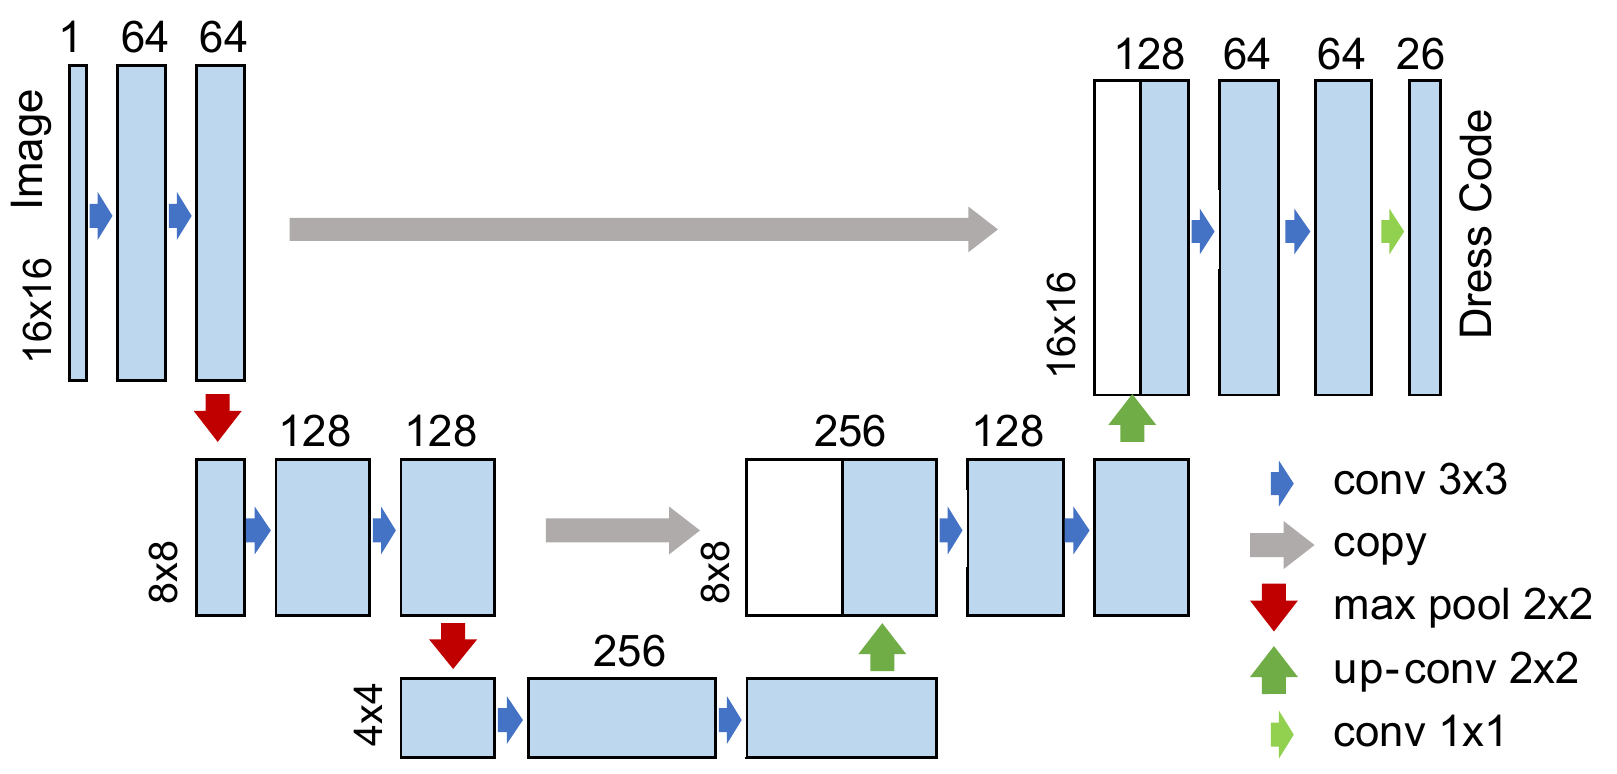}
  \caption{The network architecture of the sketch-to-pattern model.}
\end{figure}
